# Supplementary material for: Hyperparameter Tuning MLPs for Probabilistic Time Series Forecasting
Source: arXiv:2403.04477 source file (2024-03-07)
Supplement: Supplementary file 1 [file additionalresults.tex]

\clearpage
\section{Supplementary : Data}

Monash Forecasting Repository \cite{godahewa2021monash} is a collection of 50 datasets that are derived from 26 original real-world datasets by sampling time series data at different frequencies. We select 20 datasets from this collection that do not have missing values and have varying characteristics, such as length, number of series, etc., to capture the diversity of real-world time series data distributions. We evaluate our configurations on these 20 datasets. We refer the reader to Table \ref{tbl:datastat} for an in depth view of the dataset statistics. 

% Monash Forecasting Repository consists of 50 datasets derived from 26 primary real-world datasets by sampling time series data in multiple frequencies. From the 50 datasets, we evaluate configurations on 23 datasets without missing values and varying length, no. of series etc to encapsulate possible real-world time series data distributions.  
\begin{table}[]
\centering
\caption{Summary of dataset statistics used for generating the \texttt{TSBench} meta dataset.}
\resizebox{0.8\columnwidth}{!}{%
\begin{tabular}{lclcccl}
\hline
\textbf{Datasets}  & \textbf{Configs} & \textit{\textbf{Domain}} & \textit{\textbf{N\_Series}} & \textit{\textbf{Min. Len}} & \textit{\textbf{Max. Len}} & \textit{\textbf{Multi}} \\
\hline
Aus. Elecdemand    & 4860             & Energy                   & 5                           & 230736                     & 232272                     & No                      \\
Bitcoin            & 4860             & Economic                 & 18                          & 2659                       & 4581                       & No                      \\
% Electricity Hourly & 1977             & Energy                   & 321                         & 26304                      & 26304                      & Yes                     \\
% Electricity Weekly & 1948             & Energy                   & 321                         & 156                        & 156                        & Yes                     \\
FRED-MD            & 4860             & Economic                 & 107                         & 728                        & 728                        & Yes                     \\
Hospital           & 4860             & Health                   & 767                         & 84                         & 84                         & Yes                     \\
KDD                & 4860             & Nature                   & 270                         & 9504                       & 10920                      & No                      \\
M1 Monthly         & 4860             & Nature                   & 617                         & 48                         & 150                        & No                      \\
M1 Quarterly       & 4860             & Nature                   & 203                         & 18                         & 114                        & No                      \\
M1 Yearly          & 4860             & Multiple                 & 1001                        & 15                         & 150                        & No                      \\
M3 Monthly         & 4860             & Multiple                 & 1428                        & 66                         & 144                        & No                      \\
M3 Quarterly       & 4860             & Multiple                 & 756                         & 24                         & 72                         & No                      \\
M3 Yearly          & 4860             & Multiple                 & 645                         & 20                         & 47                         & No                      \\
M4 Hourly          & 4860             & Multiple                 & 414                         & 748                        & 1008                       & No                      \\
M4 Weekly          & 4860             & Multiple                 & 359                         & 93                         & 2610                       & No                      \\
NN5 Daily          & 4860             & Banking                  & 111                         & 791                        & 791                        & Yes                     \\
NN5 Weekly         & 4860             & Banking                  & 111                         & 113                        & 113                        & Yes                     \\
% Pedestrians        & 4860             & Transport                & 66                          & 576                        & 96424                      & No                      \\
Tourism Monthly    & 4860             & Transport                & 366                         & 725                        & 725                        & No                      \\
Tourism Quarterly  & 4860             & Transport                & 427                         & 91                         & 333                        & No                      \\
Tourism Yearly     & 4860             & Tourism                  & 518                         & 30                         & 130                        & No                      \\
Traffic Hourly     & 4860             & Transport                & 862                         & 17544                      & 17544                      & Yes                     \\
Traffic Weekly     & 4860             & Transport                & 862                         & 104                        & 104                        & Yes                      \\
\hline
\end{tabular}}
\label{tbl:datastat}
\end{table}
\clearpage
\section{Supplementary : Probabilistic metrics}

As presented in Table \ref{tbl:resultsCRPSmonash}, the CRPS probabilistic error metric is utilized to compare the performance of MLP models with that of DeepAR \cite{salinas2020deepar}, a well-established probabilistic forecasting model.

\begin{table}[H]
\centering
\caption{Comparison of \texttt{TSBench} results with the DeepAR model reported on the CRPS score. Best results are marked in bold. Standard deviations over multiple runs are indicated in brackets. We also provide the best overall result on the dataset across different models for reference.} 
\resizebox{0.7\columnwidth}{!}{%
\begin{tabular}{l|cc|c}
\hline
Datasets           & Train                           & Retrain                         & \multicolumn{1}{l}{\begin{tabular}[c]{@{}l@{}}DeepAR (Train) \end{tabular}}   \\
\hline
Aus. Elecdemand   & 0.068 (0.008)          & 0.064  (0.007)                            & \textbf{0.064 (0.005)}         \\
Bitcoin           & 0.572 (0.355)           & \textbf{0.264 (0.102)}                            & 0.371 (0.057)         \\
FRED-MD           & \textbf{0.034 (0.001)}          & 0.034 (0.004)                             & 0.077 (0.007)        \\
Hospital          & 0.062 (0.002)              & 0.063 (0.005)                         &  \textbf{0.050 (0.001)}         \\
KDD               & 0.447 (0.007)          & \textbf{0.447 (0.004)}                             & 0.523 (0.040) \\
M1 Monthly        & 0.187 (0.001)          & 0.178 (0.002)                             &\textbf{ 0.135 (0.007)}         \\
M1 Quarterly      & \textbf{0.090 (0.008)}           & 0.091 (0.007)                            & 0.091 (0.003)          \\
M1 Yearly         & 0.135 (0.009)          & 0.130 (0.004)                             & \textbf{0.121 (0.004)}         \\
M3 Monthly        & 0.114 (0.000)          &        -                                   & 0.099 (0.001)         \\
M3 Quarterly      & \textbf{0.066 (0.001) }         & \textbf{0.066 (0.001) }                            & 0.703 (0.000)         \\
M3 Yearly         & 0.155 (0.025)          &         -                                  & 0.117 (0.000)          \\
M4 Hourly	&0.031 (0.006) & \textbf{0.031 (0.001)} &  0.036 (0.005)\\
M4 Weekly	&\textbf{0.038 (0.001)} & 0.039 (0.000) &  0.047 (0.002)\\	
NN5 Daily	&0.134 (0.001) & \textbf{0.134 (0.000)} & 0.138 (0.002)\\	
NN5 Weekly	&0.087 (0.001) & 0.092 (0.006) & \textbf{0.075 (0.002)}  \\	
Tourism Monthly	&\textbf{0.078 (0.000)} & 0.127 (0.059) &  0.085 (0.017)\\	
Tourism Quarterly	&0.074 (0.002) & 0.072 (0.000) &\textbf{ 0.066 (0.003)} \\	
Tourism Yearly	&0.201 (0.071) & 0.242 (0.095) & \textbf{0.125 (0.002)}          \\	
Traffic Hourly	&0.224 (0.004) & \textbf{0.218 (0.003)} &  0.223 (0.00)\\	
Traffic Weekly	&0.091 (0.001) & 0.091 (0.000) & \textbf{0.087 (0.001)}	                                                                             \\
\hline
\end{tabular}}
\label{tbl:resultsCRPSmonash}
\end{table}
